# Supplementary material for: Modeling Nucleation and Growth of Zinc Oxide During Discharge of Primary Zinc-Air Batteries
Source: arXiv:1612.03464 ancillary file (2017-06-14)
Supplement: Supplementary file 1 [file Supplementary_Materials.pdf]

# Supplementary Information
# Nucleation and Growth of Zinc Oxide in Zinc-Air Button Cells

Johannes Stamm[a,b,c], Alberto Varzi[a,d], Arnulf Latz[a,b,e], Birger Horstmann[a,b]

[a] *Helmholtz Institute Ulm (HIU), Helmholtzstraße 11, 89081 Ulm, Germany*
[b] *German Aerospace Center (DLR), Institute of Engineering Thermodynamics, Pfaffenwaldring 38-40, 70569 Stuttgart, Germany*
[c] *Institute for Computational and Applied Mathematics, Universität Münster, Einsteinstraße 62, 48149 Münster, Germany*
[d] *Karlsruhe Institute of Technology (KIT), PO Box 3640, 76021 Karlsruhe, Germany*
[e] *Ulm University, Institute of Electrochemistry, Albert-Einstein-Allee 47, 89069 Ulm, Germany*

## Appendix A. Parameterization

We model the Varta PowerOne hearing aid coin cell battery PR44 type p675. Therefore, the parameters represent this battery type. Decades ago, thermodynamics and ionic transport in the aqueous alkaline electrolyte (32 weight percent KOH) were accurately studied with experiments. Thus, in Appendix A.1 we describe thermodynamic parameters and in Appendix A.2 we discuss transport parameters based on the extensive literature. In contrast, the reaction kinetics are not known with sufficient accuracy. Therefore, we choose to adjust them such that the simulated discharge curves match the measured ones (see Appendix A.3). Nevertheless, we make sure that the reaction parameters are reasonable by comparing to the literature data. We want to highlight that the qualitative features of our simulation results are robust against variations of the kinetic parameters.

Basic material parameters and physical constants are given in Tab. A.4. Experiments and Simulations are performed under standard conditions (see Tab. A.3).

In our model, the void space beneath the anode lid, which compensates the volume expansion of the active material, is distributed homogeneously along the anode (see 3.4). We adjust the volume fraction of zinc to get the observed cell capacity of 460 mAh. The (initial) volume fractions and cell dimensions are stated in Tab. A.5.

### *Appendix A.1. Thermodynamics*

#### *Appendix A.1.1. Half-Cell Potentials*

The standard half-cell potential for zinc oxidation is $\Delta\phi_{\mathrm{a}}^{0} = -1.285\mathrm{V}$ and for oxygen reduction is $\Delta\phi_{\mathrm{c}}^{0} = 0.401\mathrm{V}$ at standard conditions relative to the standard hydrogen electrode [64].

#### *Appendix A.1.2. Solubilities*

The solubility in pure water depends on the partial gas pressure by Henry's law (see Eq. 32) with Henry's constants $H_{\mathrm{O_2}}^{\mathrm{p,c}} = 7.7942 \cdot 10^4\ \mathrm{m^3Pa\ mol_{gas}^{-1}}$ and $H_{\mathrm{CO_2}}^{\mathrm{p,c}} = 2.98 \cdot 10^4\ \mathrm{m^3Pa\ mol_{gas}^{-1}}$ for oxygen and carbon dioxide, respectively [65]. At large salt concentrations (32 wt% KOH), the solubility is reduced and we must take into account salting out (see Eq. 32). The Sechenov constant is approximated as [57]

$$K^{\mathrm{s}} = \sum_i h_i c_i, \tag{A.1}$$

*Email address:* birger.horstmann@dlr.de (Birger Horstmann)

| Ion | $h_i$ / $m^3 mol^{-1}$ |
| --- | --- |
| Potassium | $0.922 \cdot 10^{-4}$ |
| Hydroxide | $0.839 \cdot 10^{-4}$ |
| Zincate | $1.423 \cdot 10^{-4}$ |
| Carbonate | $1.423 \cdot 10^{-4}$ |

Table A.1. Coefficients for Sechenov constant [57] (see Eq. A.1). The value for $ZnOH_4^=$ is chosen to be equal to the one for $CO_3^=$.

where the coefficients $h_i$ are given in Tab. A.1. At initial electrolyte concentrations, we find the solubilities $c^*_{O_2} = 13.4\ \mathrm{mol\,m^{-3}}$ and $c^*_{CO_2} = 1.1\ \mathrm{mol\,m^{-3}}$.

We calculate the solubility $c_{sat}$ of zincate depending on the potassium concentration $c_K$ [66]

$$c_{sat} = \begin{cases} -0.21 c_{std} + 0.975 \cdot 10^{-1} c_K + 0.125 \cdot 10^{-2} \frac{c_K^2}{c_{std}} & \text{if } c_K > 2.1 c_{std} \\ 0 & \text{else}\,. \end{cases} \tag{A.2}$$

Note that zinc dissolution is possible even for $c_{sat} = 0$ due to supersaturation.

*Appendix A.1.3. Molar Volumes*

The electrolyte density $\rho$ is [67]

$$\rho = \left(1024.1 + 846.6 w_1 + 307.1 w_1^2 + 1039 w_2\right) \mathrm{kg\,m^{-3}}. \tag{A.3}$$

Here, the weight percentage $w_1$ of potassium hydroxide is defined with respect to the solution $H_2O$-KOH, while that of zinc oxide $w_2$ is defined with respect to the whole electrolyte $H_2O$-KOH-ZnO.

We calculate the partial molar volumes $\bar{V}_i$ from the density in the following [61]. For this purpose, we introduce the molality $b_j := N_j m_0^{-1}$ , where $m_0$ denotes the mass of $H_2O$. The density is $\rho = m V_e^{-1}$ with the electrolyte mass $m = m_0(1 + \sum_{j=1}^{3} M_j b_j)$ and the molar masses of the salts $M_j$. Then the partial molar volume is

$$\begin{aligned} \bar{V}_j := \frac{\partial V_e}{\partial n_j} &= \frac{\partial}{\partial n_j}\left(\frac{m}{\rho}\right) = \frac{\partial}{\partial b_j}\left(\frac{1 + \sum_j M_j b_j}{\rho}\right) \\ &= -\frac{1}{\rho^2}\left(\frac{\partial \rho}{\partial b_j}\right)\left(1 + \sum_{i=0}^{3} b_i M_i\right) + \frac{1}{\rho} M_j\,. \end{aligned} \tag{A.4}$$

Molalities $b_j$ and weight percents $w_j$ are related through $w_j = w_0 b_j M_j$. By summing over all species, we find $w_0 = 1/(1 + \sum_{j=1}^{2,3} M_j b_j)$ and

$$w_j = \frac{b_j M_j}{1 + \sum_{j=1}^{2,3} M_j b_j}. \tag{A.5}$$

The sum includes ZnO for $w_2$, but not for $w_1$ here because Siu et al. define weight percent in two different ways [67].

The partial molar volume of the solvent is then determined from Eq. 44

$$\bar{V}_0 = M_0\left(\frac{1 + \sum_{j=1}^{3} M_j b_j}{\rho} - \sum_{j=1}^{3} \bar{V}_j b_j\right). \tag{A.6}$$

| Ion | Notation | Value / S $m^2mol^{-1}$ | Source |
|---|---|---|---|
| Potassium | $\lambda_{K^+}$ | $7.35 \cdot 10^{-3}$ | [64] |
| Hydroxide | $\lambda_{OH^-}$ | $19.8 \cdot 10^{-3}$ | [64] |
| Zincate | $\lambda_{Zn(OH)_4^=}$ | $9.035 \cdot 10^{-3}$ | [30] |
| Carbonate | $\lambda_{CO_3^=}$ | $6.98 \cdot 10^{-3}$ | [64] |

Table A.2. Ionic conductivity at infinite dilution

Carbonate is not included in the measurement stated in Eq. A.3. We choose to treat one $K_2CO_3$ molecules as two KOH molecules in the density calculations. Consequently, we determine its partial molar volume from that of KOH, such that the density is consistent

$$\bar{V}_{K_2CO_3} = \frac{M_{K_2CO_3}}{2M_{KOH}} \bar{V}_{KOH} \tag{A.7}$$

Note that Eq. A.3 uses the salt ZnO, but our model uses $K_2Zn(OH)_4$. The stoichiometry (see Reaction II) gives

$$\bar{V}_{K_2Zn(OH)_4^=} = 2\bar{V}_{KOH} + \bar{V}_{ZnO} + \bar{V}_{H_2O} \tag{A.8}$$

*Appendix A.2. Transport*

*Appendix A.2.1. Diffusion*

Davis et al. [69] measure and show the diffusion coefficient of oxygen in potassium hydroxide solution

$$D_{O_2} = \left[1.5 \cdot 10^{-9} \exp(-0.2878 \frac{c_{OH^-}}{c_{std}}) + 0.4 \cdot 10^{-9}\right] \frac{m^2}{s}. \tag{A.9}$$

According to May et al. [70] the diffusion coefficient of zincate depends linearly on potassium ion concentration and is independent from zincate concentration

$$D_{ZnOH_4} = \left[-9.33 \cdot 10^{-11} \frac{c_K}{c_{std}} + 1.2 \cdot 10^{-9}\right] \frac{m^2}{s}. \tag{A.10}$$

The remaining diffusion coefficients stay approximately constant in the relevant electrolyte concentration range. From literature, we find the diffusion coefficient of hydroxide [71], carbonate [72], and carbon dioxide [39] to be

$$D_{OH^-} = 3.5 \cdot 10^{-9}\, m^2s^{-1}\,, \tag{A.11}$$

$$D_{CO_3^=} = 0.82 \cdot 10^{-9}\, m^2s^{-1}\,, \tag{A.12}$$

$$D_{CO_2} = 1.5 \cdot 10^{-9}\, m^2s^{-1}\,. \tag{A.13}$$

*Appendix A.2.2. Migration*

Liu et al. [73] show that a linear mixture rule is applicable for the determination of the conductivity $\kappa$ in concentrated KOH based systems

$$\kappa = \Lambda_{KOH} c_{OH^-} + 2\Lambda_{Zn(OH)_4^=} c_{Zn(OH)_4^=} + 2\Lambda_{K2CO3} c_{CO_3^=}\,, \tag{A.14}$$

where the conductivity of binary potassium hydroxide solutions $\kappa_{KOH} = \Lambda_{KOH} c_{K^+}$ is fitted by See et al. [74] as a function of potassium concentration. The equivalent conductivities of zincate is $\Lambda_{Zn(OH)_4^=} = 7 \cdot 10^{-4}\, Sm^2mol^{-1}$ [73] and of carbonate are $\Lambda_{Zn(OH)_4^=} = (-7.14 c_{K^+}/c_{std} + 78.18) \cdot 10^{-4}\, Sm^2mol^{-1}$ [64, 73].

A definition of transference numbers for binary electrolytes is discussed in [34]. Generalizing the definition by applying the above mentioned mixture rule, the transference number of the ion species $i$ in the electrolyte with the three salts becomes

$$t_i := \frac{c_i|z_i|\lambda_i}{c_{K^+}\lambda_{K^+} + \sum_{j=1}^{3} c_j|z_j|\lambda_j}. \tag{A.15}$$

We calculate the transference numbers from the mobility at infinite dilution which are known. Values for the ionic conductivities $\lambda_i$ are given in table A.2.

We model the chemical potentials as dilute solutions and get its derivative with respect to the concentration

$$\frac{\partial\mu_i}{\partial c_i} = \frac{RT}{c_i}. \tag{A.16}$$

*Appendix A.2.3. Multi-Phase Transport*

The dynamic viscosity $\eta_e$ of aqueous potassium hydroxide solutions is given by Siu et al. [67] the permeability of the gas diffusion electrode at the initial saturation $\tilde{s}^0 = 0.63$ is $B_e = 1 \cdot 10^{-14}\,m^2$ [75]. Linear interpolating of the data in [76] yields the surface tension

$$\sigma = \left[7.2252 \cdot 10^{-5}\,\frac{m^3}{kg}\rho_e - 6.1263 \cdot 10^{-4}\right]\frac{kg}{s^2}. \tag{A.17}$$

We shift the Leverett J-function [75], such that the pressure of both, gas and liquid phase, is the standard pressure at the initial saturation $\tilde{s}^0$

$$\begin{aligned} J = {} & 1.34 \cdot 10^{-3} + 4.98 \cdot 10^{-3}\exp(9.404(\tilde{s} - \tilde{s}^0)) \\ & - 3.97 \cdot 10^{-3}\exp(-11.19(\tilde{s} - \tilde{s}^0)). \end{aligned}$$

*Appendix A.3. Reactions*

The reaction kinetics are not as accurately known as transport parameters for zinc-air batteries. Therefore, we adjust the kinetics of the two electrochemical reactions to reach quantitative agreement for the discharge curves in simulation and measurement. Nevertheless, we discuss that their orders of magnitude agree with the available literature.

*Appendix A.3.1. Zinc Morphology and Surface Areas*

We assume that spherical zinc particles are covered by a porous zinc oxide shell (see Sec. 3). This determines the specific surface areas $A_I$ for the zinc dissolution (see Eq. 25) and $A_{II}$ for the zinc oxide precipitation (see Eq. 31). The initial radius of the zinc particles is $r^0_{Zn} = 35\,\mu m$ as shown in Ref. [77]. We choose the porosity of the zinc oxide film to be $\epsilon_f = 0.05$ which is quite low, but still in agreement with Ref. [44]. We adjust the critical supersaturation to be $c_{crit} = 3.5\,c_{sat}$ according to Ref. [44].

*Appendix A.3.2. Cathode Structure and Specific Surface Areas*

The reaction surface of the oxygen and carbon dioxide absorption is the gas-liquid phase boundary in the GDE. From the lifetime experiment, we find the specific surface area $A_{III} = A_V = 3 \cdot 10^2\,m^{-1}$, which is quite low. In the cathode, zinc oxide precipitates on the active surface $A_{II} = A_{IV}$, which we keep constant during discharge. We assume that this surface coincides with the gas-liquid phase boundary $A_{IV} = 3 \cdot 10^2\,m^{-1}$.

| Name | Notation | Value | Unit |
|---|---|---|---|
| Temperature | $T$ | 298.15 | K |
| Current density | $i_{\text{cell}}$ | 100 | $\text{A m}^{-1}$ |
| Standard pressure | $p_{\text{std}}$ | 101 325 | Pa |
| Standard concentration | $c_{\text{std}}$ | 1 000 | $\text{mol m}^{-3}$ |
| Partial pressure oxygen | $p_{O_2^g}$ | 21 219 | Pa |
| Partial pressure carbon dioxide | $p_{CO_2^g}$ | 39 | Pa |
| Standard oxygen concentration | $c_{O_2,\text{std}}$ | 0.867 | $\text{mol m}^{-3}$ |

Table A.3. Conditions for experiment and simulation. The partial gas pressures represent ambient air and are taken from Ref. [68]. The standard oxygen concentration corresponds to equilibrium with oxygen gas at standard pressure.

### *Appendix A.3.3. Kinetic Coefficients*

We adjust the kinetic constant $k_{\text{I}} = 1.8 \cdot 10^{-6}\ \text{mol m}^{-2}\text{s}^{-1}$ (cf. [32]) for zinc dissolution. At typical concentrations, this value corresponds to the exchange current density $i_0 \approx 1\ \text{Am}^{-2}$. This value is two orders of magnitude lower than measured on pure zinc [30]. Modern zinc anodes, however, contain additives in order to suppress hydrogen evolution. These additives can also slow down zinc dissolution.

Our adjusted kinetic coefficient for oxygen reduction $k_{\text{IV}} = 3 \cdot 10^{-10}\ \text{mol m}^{-2}\text{s}^{-1}$ corresponds to the exchange current $i_0 \approx 10^{-4}\ \text{Am}^{-2}$. This results in the exchange current density $i_0^{\text{GDE}} \approx 10^{-5}\ \text{Am}^{-2}$ with respect to the cross-section of the whole GDE in approximate agreement with the measurements of Drillet et al. for carbon based gas diffusion electrodes coated with $MnO_2$ [78].

The kinetic constant $k_{\text{III}}$ of oxygen dissolution follows from the Hertz-Knudsen equation 33. We assume that one percent $\xi := 0.01$ of the gas molecules hitting the gas-liquid phase boundary enter the electrolyte [12]. The kinetics of ZnO growths is determined by the diffusion layer thickness $\delta_{\text{ZnO}} = 1\,\mu\text{m}$ resulting in kinetics similar to previous models [32, 25].

The kinetic coefficient of the carbonate reaction $k_V := k_{\text{OH}^-} c_{\text{OH}^-}$ (see Eq. 37) follows from the kinetic constant $k_{\text{OH}^-}$ of the rate determining step (see Reaction V.a) [79]

$$k_{\text{OH}^-} = 8.38 \frac{\text{mol}}{\text{m}^3\text{s}} \cdot 10^{(0.11 c_{\text{K}^+} + 0.11 c_{\text{OH}^-} + 0.17 c_{\text{CO}_3^=})/c_{\text{std}}}. \tag{A.18}$$

### *Appendix A.4. Initial Conditions*

The initial conditions are given in Tab. A.6. Varta PowerOne hearing aid batteries PR44 type p675 contain 32 wt% potassium hydroxide electrolyte. Accordingly, we choose the concentrations of water and potassium. For numerical reasons we set small initial concentrations for carbonate and zincate. Then we calculate the hydroxide concentration, such that charge neutrality is granted.

In our model the void space on top of the anode is homogeneously distributed throughout the cell. The volume fraction of zinc is adjusted to give the observed cell capacity of 460 mAh (see Tab. A.5). The initial zinc particle radius is $r_{\text{Zn}}^0 = 35\,\mu\text{m}$ [77].

| Name | Notation | Value | Unit |
|---|---|---|---|
| Ideal gas constant | $R$ | 8.3144 | $J\,mol^{-1}K^{-1}$ |
| Faraday constant | $F$ | 96485 | $C\,mol^{-1}$ |
| Boltzmann constant | $k_B$ | $1.3806488 \cdot 10^{-23}$ | $m^2kg\,s^{-2}K^{-1}$ |
| Molar mass | | | |
| Water | $M_{H_2O}$ | $18.015 \cdot 10^{-3}$ | $kg\,mol^{-1}$ |
| Potassium | $M_K$ | $39.0983 \cdot 10^{-3}$ | $kg\,mol^{-1}$ |
| Oxygen | $M_{O_2}$ | $31.9988 \cdot 10^{-3}$ | $kg\,mol^{-1}$ |
| Hydroxide | $M_{OH^-}$ | $17.00734 \cdot 10^{-3}$ | $kg\,mol^{-1}$ |
| Zincate | $M_{ZnOH_4^=}$ | $133.4094 \cdot 10^{-3}$ | $kg\,mol^{-1}$ |
| Carbon dioxide | $M_{CO_2}$ | $44.0095 \cdot 10^{-3}$ | $kg\,mol^{-1}$ |
| Density Water | $\rho_{H_2O}$ | 997.048 | $kg\,m^{-3}$ |
| Molar volume zinc | $V_{Zn}$ | $9.16 \cdot 10^{-6}$ | $m^3mol^{-1}$ |
| Molar volume zinc oxide | $V_{ZnO}$ | $14.5 \cdot 10^{-6}$ | $m^3mol^{-1}$ |

Table A.4. Basic material parameters and physical constants [64].

| Name | Notation | Ano. | Sep. | Cat. | Unit |
|---|---|---|---|---|---|
| Cell diameter | | | $11 \cdot 10^{-3}$ | | m |
| Length | $L_a$,$L_s$,$L_c$ | $4.5 \cdot 10^{-3}$ | $0.1 \cdot 10^{-3}$ | $0.3 \cdot 10^{-3}$ | m |
| Volume fraction | | | | | |
| Zinc | $\epsilon^0_{Zn}$ | 0.185 | - | - | - |
| Zinc oxide | $\epsilon^0_{ZnO}$ | $1{\cdot}10^{-7}$ | $1{\cdot}10^{-7}$ | $1{\cdot}10^{-7}$ | - |
| Inactive material | $\epsilon^0_{inact}$ | - | 0.185 | 0.185 | - |
| Electrolyte | $\epsilon^0_e$ | 0.515 | 0.515 | 0.515 | - |
| Gas phase | $\epsilon^0_g$ | 0.3 | 0.3 | 0.3 | - |
| Initial zinc particle diameter | $r^0_{Zn}$ | 75 | | | $\mu$m |

Table A.5. Geometry for simulating the VARTA PowerOne button cell PR44 type p675.

| Name | Notation | Value | Unit |
|---|---|---|---|
| Density electrolyte | $\rho^0_e$ | 1301 | $kg\,m^{-3}$ |
| Concentration | | | |
| Water | $c^0_{H_2O}$ | 49105 | $mol\,m^{-3}$ |
| Potassium | $c^0_{K^+}$ | 7419.9 | $mol\,m^{-3}$ |
| Oxygen | $c^0_{O_2}$ | 0.0134 | $mol\,m^{-3}$ |
| Hydroxide | $c^0_{OH^-}$ | 7417.9 | $mol\,m^{-3}$ |
| Zincate | $c^0_{ZnOH_4^=}$ | 1 | $mol\,m^{-3}$ |
| Carbonate | $c^0_{CO_3^=}$ | $10^{-8}$ | $mol\,m^{-3}$ |

Table A.6. Initial conditions for electrolyte composition at 32wt% KOH.

## Appendix B. Experimental Sequence

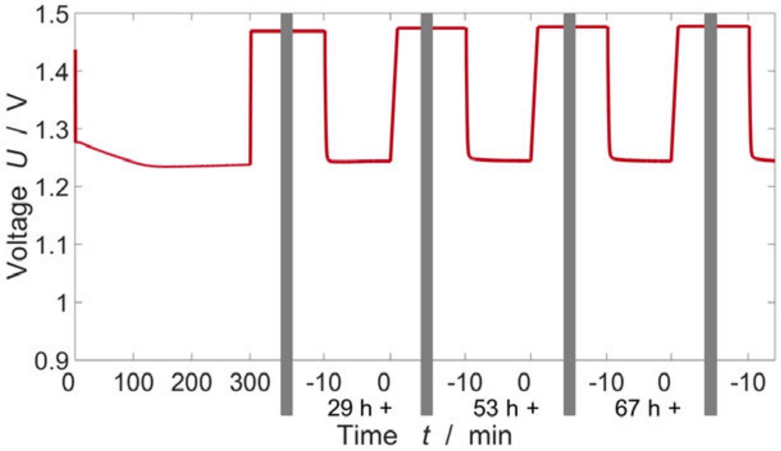


Figure B.1. Lifetime analysis at 100 $Am^{-2}$. The voltage is shown as a function of measurement time. After an initial discharge for 5 h, the cell is discharged for ten minutes every day. The figure depicts the measurement in the first four days, the gray arrays separate the measurements on different days.

## Appendix C. Carbon Dioxide Filter

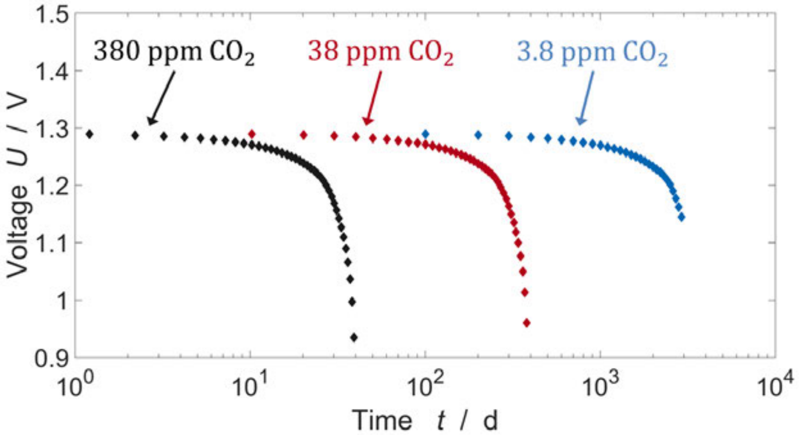


Figure C.2. Simulated lifetime analysis at 100 $Am^{-2}$. The voltage is shown as a function of measurement time. The discharge proceeds with varying carbon dioxide content in the feed gas. The voltage is measured every 24h, 240h, 2400h for 380ppm $CO_2$, 38ppm $CO_2$, 3.8ppm $CO_2$, respectively. We find that the lifetime is approximately inversely proportional to the carbon dioxide content.

## Appendix D. Battery Cycling

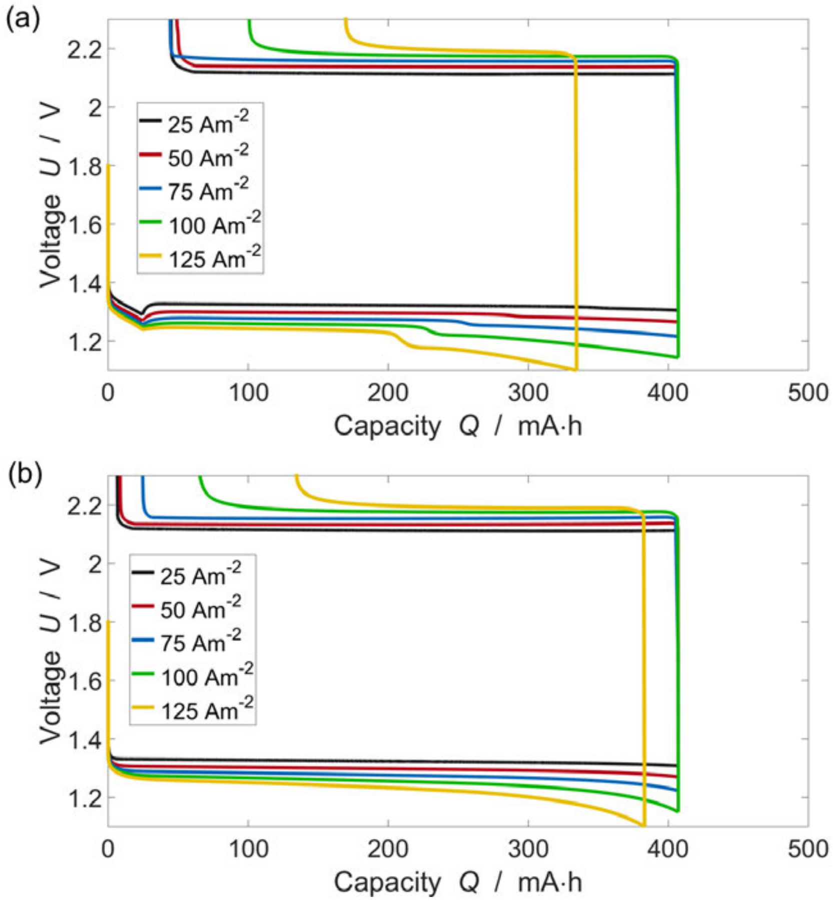


Figure D.3. Simulated voltage curves during discharge and charge as a function of discharged capacity at various current densities. The discharge proceeds to 90% capacity $Q$ = 407 mAh or to the voltage cut-off at $U$ = 1.1 V. The initial anode consists of (a) pure Zn and (b) a mixture of 2 volume percent ZnO and 98 volume percent Zn.
